# Supplementary material for: SwiftRL: Towards Efficient Reinforcement Learning on Real Processing-In-Memory Systems
Source: arXiv:2405.03967 source file (2024-05-07)
Supplement: Supplementary file 1 [file Q_SARSA_combined.tex]

\documentclass{article}
\usepackage{algorithm}
\usepackage{algpseudocode}
\usepackage{amsmath}

\begin{document}

\begin{algorithm}
\caption{Offline Tabular RL with Batch Updates}
\begin{algorithmic}
\State \textbf{Initialization:}
\State Read the experience data.
\State Initialize Q-table with arbitrary/zero values.
\State Define hyperparameters: Learning Rate ($\alpha$), Discount Factor ($\gamma$), Number of Iterations, Batch Size.
\State $\alpha, \gamma, \text{Number of Iterations}, \text{Batch Size}$

\State \textbf{Offline Data:}
\State Use offline data from past experiences.

\For {iteration from 1 to Number of Iterations}
    \State \textbf{Select Batch Data for Iteration:}
    \State Choose a batch of experiences for this iteration.

    \For {each batch window from 1 to total batch windows}
        \State \textbf{Q-Value Update (Q-learning):}
        \For {each experience in selected batch}
            \State Calculate Q-value target for the experience:
            \State \small $q_{\text{value target}} = \text{reward} + \gamma \cdot \max(Q[\text{next\_state}])$
            \State Update Q-values for the current state-action pair:
            \State $Q[\text{state}][\text{action}] = Q[\text{state}][\text{action}] + \alpha \cdot (q_{\text{value target}} - Q[\text{state}][\text{action}])$
        \EndFor

        \State \textbf{SARSA Update:}
        \For {each experience in selected batch}
            \State Calculate SARSA target for the experience:
            \State \small $sarsa_{\text{target}} = \text{reward} + \gamma \cdot Q[\text{next\_state}][\text{next\_action}]$
            \State Update Q-values for the current state-action pair:
            \State $Q[\text{state}][\text{action}] = Q[\text{state}][\text{action}] + \alpha \cdot (sarsa_{\text{target}} - Q[\text{state}][\text{action}])$
        \EndFor
    \EndFor
\EndFor

\State \textbf{Result:}
\State Final Q-table with the learned Q-values.

\end{algorithmic}
\end{algorithm}

\end{document}
