# Supplementary material for: SwiftRL: Towards Efficient Reinforcement Learning on Real Processing-In-Memory Systems
Source: arXiv:2405.03967 source file (2024-05-07)
Supplement: Supplementary file 3 [file Toy.tex]

\documentclass{article}
\usepackage{pgfplots}
\pgfplotsset{compat=newest}

\begin{document}

\begin{tikzpicture}
\begin{axis}[
    title={Roofline Model},
    xlabel={Arithmetic Intensity},
    ylabel={Performance (GOPS)},
    xmin=0, xmax=10,
    ymin=0, ymax=100,
    legend pos=north west,
    grid style=dashed,
]

% L1 Bandwidth
\addplot[
    color=blue,
    mark=square,
    ]
    coordinates {
    (0,20)(5,20)
    };
\addlegendentry{L1 Bandwidth}

% L2 Bandwidth
\addplot[
    color=red,
    mark=square,
    ]
    coordinates {
    (0,40)(5,40)
    };
\addlegendentry{L2 Bandwidth}

% L3 Bandwidth
\addplot[
    color=green,
    mark=square,
    ]
    coordinates {
    (0,60)(5,60)
    };
\addlegendentry{L3 Bandwidth}

% DRAM Bandwidth
\addplot[
    color=orange,
    mark=square,
    ]
    coordinates {
    (0,80)(5,80)
    };
\addlegendentry{DRAM Bandwidth}

% Compute Bound Line
\addplot[
    domain=0:10,
    samples=100,
    color=black,
    ]
    {x*10};
\addlegendentry{Compute Bound}

\end{axis}
\end{tikzpicture}

\end{document}
